# Supplementary material for: Atomistic simulations of athermal irradiation creep and swelling of copper and tungsten in the high dose limit
Source: arXiv:2409.13355 ancillary file (2024-09-20)
Supplement: Supplementary file 1 [file SupplMat_Reali_et_al_2024.pdf]

# Supplementary Material to: Atomistic simulations of athermal irradiation creep and swelling of copper and tungsten in the high dose limit

Luca Reali,* Max Boleininger,† Daniel R. Mason,‡ and Sergei L. Dudarev§
*United Kingdom Atomic Energy Authority, Culham Campus, Oxfordshire OX14 3DB, UK*

## I. DESCRIPTION OF THE ALGORITHM

Here, we provide a detailed description of the molten spheres algorithm briefly summarised in the main text of the paper. Before generating an irradiated configuration, a single simulation is run to bring the simulation cell to a molten configuration; the coordinates of the atoms in the liquid phase are stored. About 1 and 2 million atoms were used for W and Cu.

The simulation starts from a pristine lattice after the box was allowed to relax to the minimum energy configuration under the constant applied external stress. Irradiation is then simulated with the dose increment of $\sim 10^{-4}$ dpa per step. This value was chosen to be similar to the one used in the overlapping cascades simulations [1]. The number of spheres inserted at each step, $N$, depends on the primary knock-on atom (PKA) energy defined according to the relation between the radius $R$ of a molten region and the damage energy that defined in Fig. 1 of the main paper. $N$ spherical regions are defined at each algorithmic step of the simulation, each containing a number of atoms close to $4\pi n R^3/3$, where $n$ is the atomic density. The atoms in the selected spherical regions are then deleted. For instance, the $i$-th sphere may contain $N_i$ atoms. The closest $N_i$ atoms from a randomly selected atom of the molten configuration are selected, thereby defining a spherical molten region. $N$ such regions are defined and inserted in place of the deleted atom regions, taking care to ensure that the number of atoms is conserved. The system then is subjected to energy minimisation under applied external stress, to recrystallise the molten regions and allow for the re-organisation of the defects. Energy is minimised using a relative convergence threshold of $10^{-12}$, in other words LAMMPS is set to adjust the atomic coordinates to decrease the total potential energy until the change in the energy in one iteration divided by its magnitude is less than $10^{-12}$. The process is repeated until the desired dose is reached. Before each insertion step, the entire lattice is shifted by a random distance in all three directions to ensure there are no artefacts introduced in having no melting of the atoms very close to the periphery of the box.

In the case of a single PKA energy all the spheres are identical. A *spectrum* of PKA energies can be simulated as well by simply drawing the equivalent radii from a suitable distribution.

### A. Efficiency considerations

The molten sphere algorithm is intended to provide a trade-off between the creation relaxation algorithm (CRA) [2, 3], very fast and easy to implement but predicting too high defect concentrations, and the repeated simultaneous initiation of full collision cascades in molecular dynamics (MD) [4]. Another possible trade-off in-

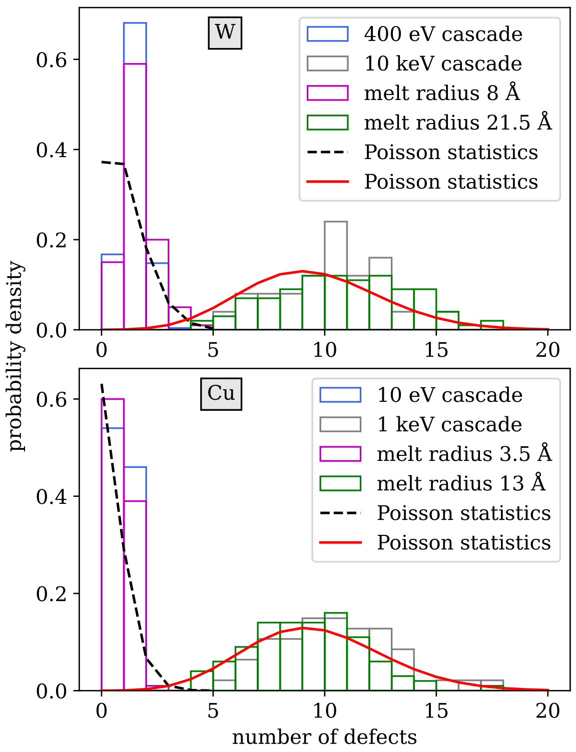


FIG. S1. Normalised histogram of the number of surviving Frenkel pairs generated using either full cascade simulations or recrystallising molten spheres corresponding to similar equivalent energies. The statistical distributions are similar in W and Cu, both for the low and high energy recoils. Poisson distributions are also shown; the expected value or shape parameter of the distributions were taken to be the mean of the cascade data.

* Luca.Reali@ukaea.uk
† Max.Boleininger@ukaea.uk
‡ Daniel.Mason@ukaea.uk
§ Sergei.Dudarev@ukaea.uk

volves combining CRA and MD (CRA+MD), which produces results similar to a full MD simulation but requires a fraction of the simulation time [5].

## II. COMPARISON WITH COLLISION CASCADES AND EXPERIMENTS

### A. Single cascade

Fig. 1 of the main text shows that the molten spheres algorithm is able to reproduce the number of point defects surviving a collision cascade over a broad range of $E_{\mathrm{PKA}}$. Here, we also consider how the two methods compare in terms of the distribution of numbers of defects. If a single occurrence of a cascade or the recrystallisation of a single molten sphere creates $N$ Frenkel pairs, what is the distribution of $N$ if the process is repeated many times? We considered one low energy and one high energy case in W and in Cu. For W we considred low energy collision cascades of $E_{\mathrm{PKA}} = 400$ eV, corresponding to the displacement energy of 351 eV, while for Cu we assumed $E_{\mathrm{PKA}} = 10$ eV, approximately same as the displacement energy. For the high energy, $E_{\mathrm{PKA}}$ values of 10 keV and 1 keV were selected, corresponding to damage energies of 8022 eV and 820 eV respectively. Damage energies of the molten spheres, for comparison, corresponded to 365 eV and 7090 eV in W—using spheres of radius 8 Å and 21.5 Å — and 9.6 and 491 eV in Cu, using spheres of radius 3.5 Å and 13 Å. The data shown in the Figure also include the Poisson statistics, with a shape parameter, or the mean, given by the mean value of the cascade data sample. We found that the Poisson distribution better describes the high-energy recoils statistics or, equivalently, larger molten spheres. In fact, the $\chi^2$-test showed that the hypothesis that the data follow a Poisson distribution should be rejected with a $p$-value $p < 0.05$ for both the W and Cu low-energy data shown in Fig. S1. The same hypothesis should be accepted, on the other hand, for the high-energy data with $p > 0.10$. The results for true cascades and recrystallised molten spheres were similar.

### B. Overlapping 10 keV cascades in W

In Ref. [4], several 10 keV cascades were simultaneously initiated in a 21-million atom W box to reach 1 dpa in $2 \cdot 10^{-4}$ dpa steps. Here, an analogous simulation was performed by inserting molten spheres having a radius of 24 Å and recrystallising the material. Fig. S2 compares the two methods in terms of the total volumetric swelling, vacancy concentration, and the total dislocation density. Qualitatively the results are similar, although the molten sphere method produces about 25 % more defects. This is likely due to the absence of localised heating caused by the thermal spike that favours partial self-annihilation of the defects.

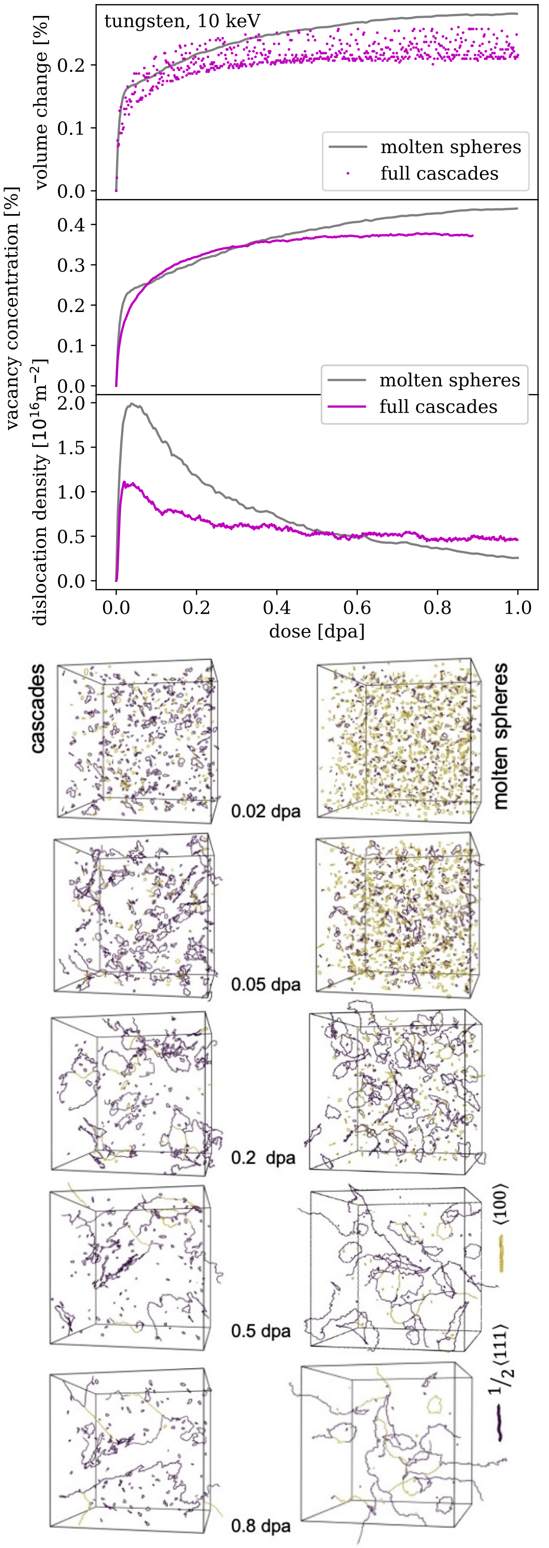


FIG. S2. Comparison between swelling, vacancy content and DXA analysis from the molten sphere method and full ballistic MD simulation of 10 keV recoils in W (the data for the latter are taken from Ref. [4]).

TABLE S1. Qualitative comparison of features and computational requirements for the four methods for athermally generating high-dose microstructures. These are: the molten sphere algorithm (MSA) as implemented in this study, the creation relaxation algorithm (CRA) [2], the combination of CRA and single overlapping cascades in MD [5], and multiple overlapping cascades in MD [4]. All the simulation methods require sequential steps that may either be the minimisation steps of a conjugate gradient algorithm or time-steps for integration of the equations of motion of the atoms, which we assume take the same time per step in a computer. To be roughly independent of the simulation size, we consider a number of MD steps here; in the limit of ideal parallel scaling the wall-time is given by multiplying the steps/dpa times the time/step which depends on the number of cores dedicated to the simulation.

| method | speed [$10^6$ steps/dpa] | advantages | disadvantages |
|---|---|---|---|
| MD | 200 | can simulate a spectrum of recoils | computational cost |
| MSA | 20 | can simulate a spectrum of recoils | slight overestimation of defect content (x1.5) |
| CRA | 10 | easy implementation | severe overestimation of defect content (x10)<br>cannot simulate a spectrum of recoils |
| CRA+MD | 20 | anneals excess CRA damage to same as MD<br>at low computational cost<br>accurate high dose microstructure | cannot represent continuous dose evolution<br>cannot simulate continuous dose<br>number of steps scales proportional to volume |

## C. Ion-irradiated tungsten foil

Ref. [6] shows a comparison between experimental measurements of lattice strain and a CRA simulation. Tungsten was irradiated with 20.3 MeV tungsten ions and the lattice strain $\varepsilon_{zz}$ normal to the foil surface was measured. $\varepsilon_{zz}$ was found to grow in the low-dose limit, to reach a maximum at about 0.03 dpa, and then decreases to negative values of strain of about the same magnitude. The zero strain was observed at about 0.1 dpa and saturation was reached after 1 dpa. Simulations [6] exhibited the same trend but with an overestimation by about a factor of 10.

We simulated a 128x128x400 W supercell containing 13,107,200 atoms until about 2 dpa in 0.0004 dpa steps. Importantly, The radii of the molten spheres were drawn from a distribution that replicated the distribution of recoil energy obtained using the SRIM code [1]. Fig. S3 compares the experimental data from [6] and our simulation. With respect to the Frenkel pair accumulation CRA simulations, the overestimation of experimental data is reduced to about a factor of 1.5-2. The qualitative agreement is very good. Similarly to Ref. [6], $\varepsilon_{zz}$ was calculated based on the shift in position of the [002] spot of a simulated diffraction pattern.

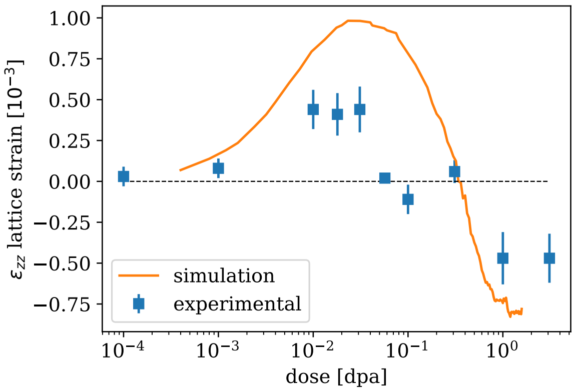


FIG. S3. The lattice strain $\varepsilon_{zz}$ normal to the surface of W irradiated at low temperature with 20.3 MeV ions was experimentally characterised in Ref. [6]. The radii of molten spheres were drawn from the corresponding $E_{\mathrm{PKA}}$ spectrum

## III. UNCERTAINTY QUANTIFICATION

To quantify the uncertainty of the results that were presented in the main text, we selected one case for W, namely uniaxial tension under 7 keV recoils, and one for Cu, uniaxial tension under 5 keV recoils. Five simulations with identical initial setup were run in each case. The resulting hydrostatic and von Mises strains are shown in Fig. S4a for W and Fig. S4b for Cu. A band corresponding to ± one standard error is added to the mean curves. The scatter of the hydrostatic strain was barely noticeable and less than 1 %. The standard error of the von Mises strain was greater, but still about 10 % of the mean value. Additionally, also the eigenvectors of the strain tensor at 1 dpa are shown in comparison to the 0 dpa eigenvectors, where the principal eigenvector points exactly along $z$.

The vacancy concentration and the dislocation density are shown in Fig. S4c and Fig. S4d respectively, showing low uncertainty comparable to the one found for the hydrostatic strain. On the basis of these results, we conclude that the degree of uncertainty in these simulations is not high, being higher for the deviatoric part of swelling than for the hydrostatic part.

Fig. S4 addresses the variability of results derived from repeated simulations. There is also a source of uncertainty that affects the definition of dose. We recall that the dose after inserting $N_{\mathrm{tot}}$ spheres was defined in the main text as

$$\phi = N_{\mathrm{tot}} \frac{0.8}{2E_{\mathrm{d}}N_{\mathrm{el}}} \frac{4\pi}{3} \frac{R^3}{\Omega_0} E_{\mathrm{melt}}. \quad (1)$$

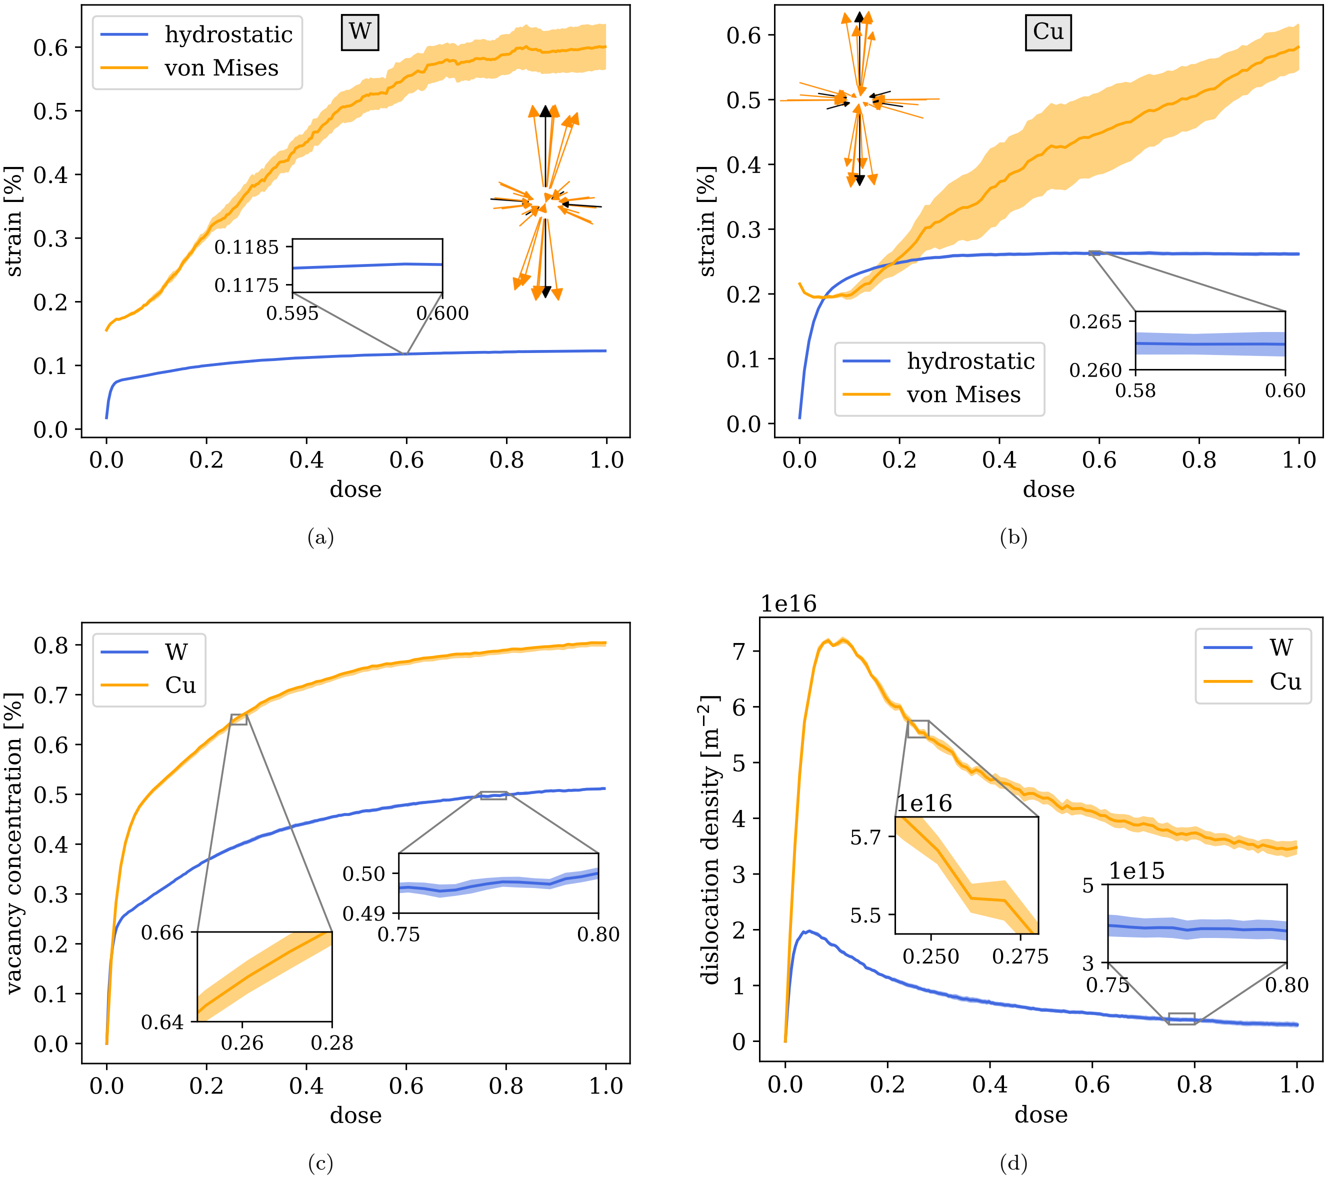


FIG. S4. Simulations of uniaxial tension under high-energy irradiation were repeated over five independent runs to quantify the uncertainty of the results, shown here as average with ± one standard error band. The standard error of the supercell hydrostatic strain of W (a) and Cu (b), as well as the vacancy concentration (c) showed less than 1 % variation. The dislocation density (d) was only slightly more uncertain. Only the von Mises strain showed a noticeable standard error of about 10 % of the mean value. In (a) and (b) black arrows indicate the normalised eigenvectors of the strain tensor at the start of the simulation. 5 sets of orange arrows indicate the same eigenvectors at the end of the simulation, 1 dpa. In all cases the deformation of the box evolved closely following the initial elastic deflection even if the magnitude of the von Mises strain grew by about a factor of 3 to 4.

There is therefore an uncertainty that is entirely contained in the ratio $E_{\mathrm{melt}}/E_{\mathrm{d}}$. If the uncertainty on $E_{\mathrm{melt}}$ is low (see Supplementary Material of [1]), $E_{\mathrm{d}}$ is a scalar used to represent an anisotropic quantity. For instance, in W the minimum value is as low as about 40 eV whereas the maximum is above 200 eV, with values of $E_{\mathrm{d}}$ given at about 90 to 100 eV [1, 7]. However, dose here is to be intended as a conventional measure of exposure, rather than a quantification of damage. In our case we selected $E_{\mathrm{d}} = 90$ eV. Finally, it is important to remember that, as with every molecular dynamics simulation, there is an intrinsic error introduced by the choice of the interatomic potential.

## IV. STRAIN ANALYSIS AND ELASTO-PLASTIC DECOMPOSITION

The MD supercell of a non-orthogonal simulation box is defined by LAMMPS using matrix $\mathbf{A}$

$$\mathbf{A}=\begin{bmatrix}a_x & b_x & c_x\\ 0 & b_y & c_y\\ 0 & 0 & c_z\end{bmatrix}$$

containing the basis vectors $\mathbf{a}$, $\mathbf{b}$ and $\mathbf{c}$ in the three columns. Regardless of the deformation of the cell, $\mathbf{a}$ is kept aligned with the positive $x$ axis and $\mathbf{a}$ is kept inside the $xy$ plane.

A general initial configuration is $\mathbf{A^0}$ with $\mathbf{a^0}=[a_x^0,0,0]$, $\mathbf{b^0}=[b_x^0,b_y^0,0]$ and $\mathbf{c^0}=[c_x^0,c_y^0,c_z^0]$. After some deformation of the box due to irradiation and applied stress, let the supercell be defined by matrix $\mathbf{A}$ above. The supercell strain after deformation can be thought of as a transformation of the initial supercell, *via* the transformation encoded in the deformation gradient tensor $\mathbf{F}$. Considering the three basis vectors independently gives

$$\begin{aligned}\mathbf{a}&=\mathbf{F}\cdot\mathbf{a^0}\\ \mathbf{b}&=\mathbf{F}\cdot\mathbf{b^0}\\ \mathbf{c}&=\mathbf{F}\cdot\mathbf{c^0}.\end{aligned}\tag{2}$$

Since the deformed and original configurations are known, we solve for the components of $\mathbf{F}$

$$\begin{aligned}&F_{xx}=\frac{a_x}{a_x^0} \quad F_{xy}=\frac{b_x}{b_y^0}-\frac{a_xb_x^0}{a_x^0b_y^0} \quad F_{xz}=\frac{c_x}{c_z^0}-\frac{a_xc_x^0}{a_x^0c_z^0}-\left(\frac{b_x}{b_y^0}-\frac{a_xb_x^0}{a_x^0b_y^0}\right)\frac{c_y^0}{c_z^0}\\ &F_{yx}=0 \quad F_{yy}=\frac{b_y}{b_y^0} \quad F_{yz}=\frac{c_y}{c_z^0}-\frac{b_yc_y^0}{b_y^0c_z^0}\\ &F_{zx}=0 \quad F_{zy}=0 \quad F_{zz}=\frac{c_z}{c_z^0}.\end{aligned}$$

If, like in our case, the box starts from an orthogonal configuration having $b_x^0=c_x^0=c_y^0=0$ we have a greatly simplified tensor

$$\mathbf{F}=\begin{bmatrix}\frac{a_x}{a_x^0} & \frac{b_x}{b_y^0} & \frac{c_x}{c_z^0}\\ 0 & \frac{b_y}{b_y^0} & \frac{c_y}{c_z^0}\\ 0 & 0 & \frac{c_z}{c_z^0}.\end{bmatrix}\tag{3}$$

Recalling that the Green-Lagrangian strain tensor tensor for a given deformation gradient is

$$\boldsymbol{\varepsilon}=\frac{1}{2}\left(\mathbf{F^TF}-\mathbf{I}\right),\tag{4}$$

where $\mathbf{I}$ is the identity tensor, we find the six strain components in terms of deformed and initial simulation box:

$$\varepsilon_{xx}=\frac{1}{2}\left[\left(\frac{a_x}{a_x^0}\right)^2-1\right]\tag{5}$$

$$\varepsilon_{yy}=\frac{1}{2}\left[\left(\frac{b_x}{b_y^0}\right)^2+\left(\frac{b_y}{b_y^0}\right)^2-1\right]\tag{6}$$

$$\varepsilon_{zz}=\frac{1}{2}\left[\left(\frac{c_x}{c_z^0}\right)^2+\left(\frac{c_y}{c_z^0}\right)^2+\left(\frac{c_z}{c_z^0}\right)^2-1\right]\tag{7}$$

$$\varepsilon_{xy}=\frac{1}{2}\left[\frac{a_x}{a_x^0}\frac{b_x}{b_y^0}\right]\tag{8}$$

$$\varepsilon_{yz}=\frac{1}{2}\left[\frac{b_x}{b_y^0}\frac{c_x}{c_z^0}+\frac{b_y}{b_y^0}\frac{c_y}{c_z^0}\right]\tag{9}$$

$$\varepsilon_{xz}=\frac{1}{2}\left[\frac{a_x}{a_x^0}\frac{c_x}{c_z^0}\right].\tag{10}$$

Although for calculating our results we used the finite strain definitions, we can check that in the limit of small deviations from the undeformed configuration the above definitions yield the expected small-strain definitions. Indicating with $\delta$ an infinitesimal deviation from the starting cell vectors we have that $a_x=a_x^0+\delta a_x$, $b_y=b_y^0+\delta b_y$, $c_z=c_z^0+\delta c_z$, $b_x=\delta b_x$, $c_x=\delta c_x$, $c_y=\delta c_y$ and the small strain tensor becomes

$$\begin{aligned}&\varepsilon_{xx}=\frac{\delta a_x}{a_x^0} \quad \varepsilon_{xy}=\frac{1}{2}\frac{\delta b_x}{b_y^0} \quad \varepsilon_{xz}=\frac{1}{2}\frac{\delta c_x}{c_z^0}\\ &\varepsilon_{yy}=\frac{\delta b_y}{b_y^0} \quad \varepsilon_{yz}=\frac{1}{2}\frac{\delta c_y}{c_z^0}\\ &\varepsilon_{zz}=\frac{\delta c_z}{c_z^0}.\end{aligned}$$

From the supercell strain tensor we calculate the hydrostatic and von Mises strains. We also recall that the definition of the von Mises strain in terms of components of strain tensor $\varepsilon_{ij}$ is

$$\varepsilon_{\mathrm{vM}}=\frac{1}{\sqrt{2}}\Big((\varepsilon_{xx}-\varepsilon_{yy})^2+(\varepsilon_{yy}-\varepsilon_{zz})^2+(\varepsilon_{zz}-\varepsilon_{xx})^2+6(\varepsilon_{xy}+\varepsilon_{yz}+\varepsilon_{xz})^2\Big)^{1/2}.\tag{11}$$

Alternatively, if the deviatoric strain is calculated as $\varepsilon_{ij}^{\mathrm{d}}=\varepsilon_{ij}-\frac{1}{3}\varepsilon_{kk}\delta_{ij}$, the von Mises strain is given by $\varepsilon_{\mathrm{vM}}=\sqrt{\frac{3}{2}\varepsilon_{ij}^{\mathrm{d}}\varepsilon_{ij}^{\mathrm{d}}}$. Fig. S5 summarises the evolution, as a function of dose, of the hydrostatic and deviatoric strains for the simulations presented in this work: high- and low equivalent recoil energy irradiation in tungsten and copper.

From the total deformation gradient $\mathbf{F}$ we determine the total box strains. $\mathbf{F}$ is multiplicatively given by the elastic part $\mathbf{F^e}$, which is the one giving rise to elastic stress, and by the inelastic part. In general the inelastic part contains the plastic contribution and swelling, $\mathbf{F}^\omega$ and $\mathbf{F}^\omega$ respectively. In the athermal limit that we are exploring, this irreversible deformation is caused by irradiation-induced tensorial swelling and we assume that $\mathbf{F}^\omega=0$. By comparing the deformed supercell vectors and the initial supercell vectors we have that

$$\mathbf{A}=\mathbf{F}^{\mathrm{el}}\mathbf{F}^{\omega}\mathbf{A^0}\equiv(\mathbf{1}+\boldsymbol{\varepsilon}^{\mathrm{el}})\mathbf{R}(\mathbf{1}+\boldsymbol{\varepsilon}^{\boldsymbol{\omega}})\mathbf{A^0},\tag{12}$$

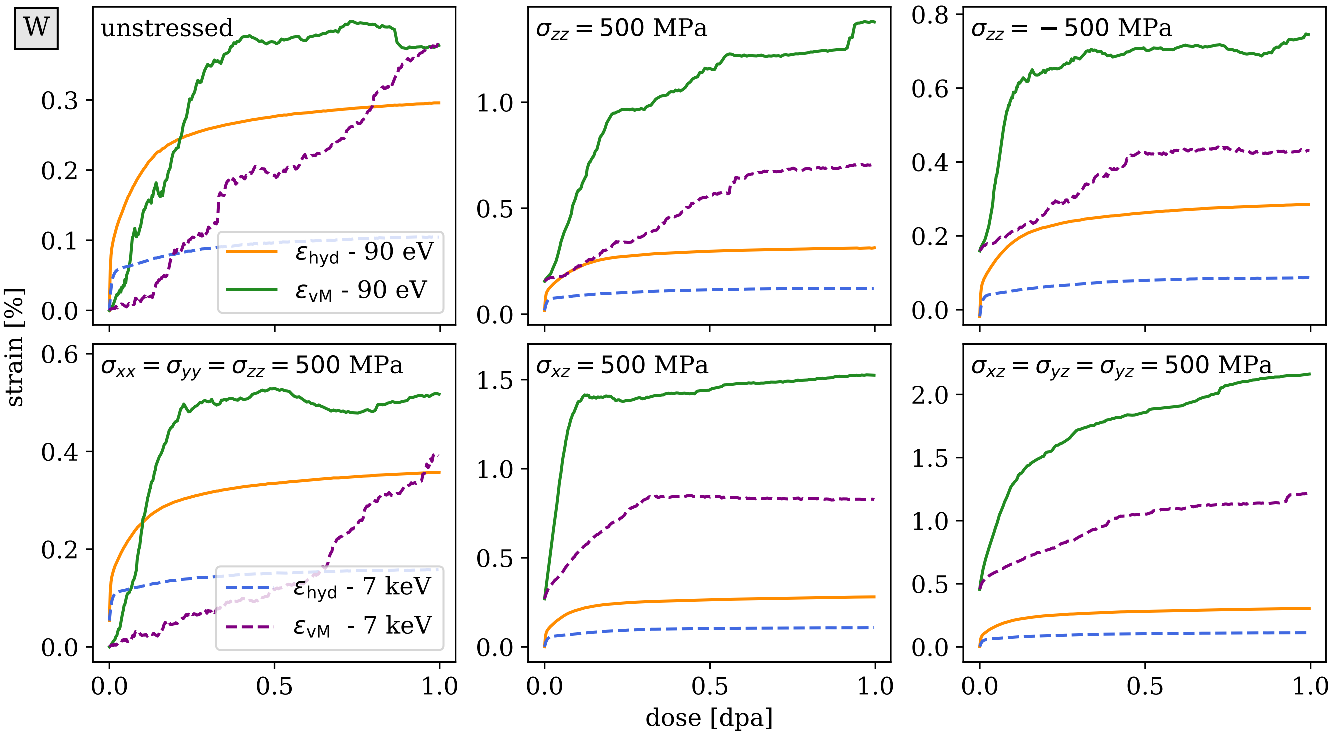


(a)

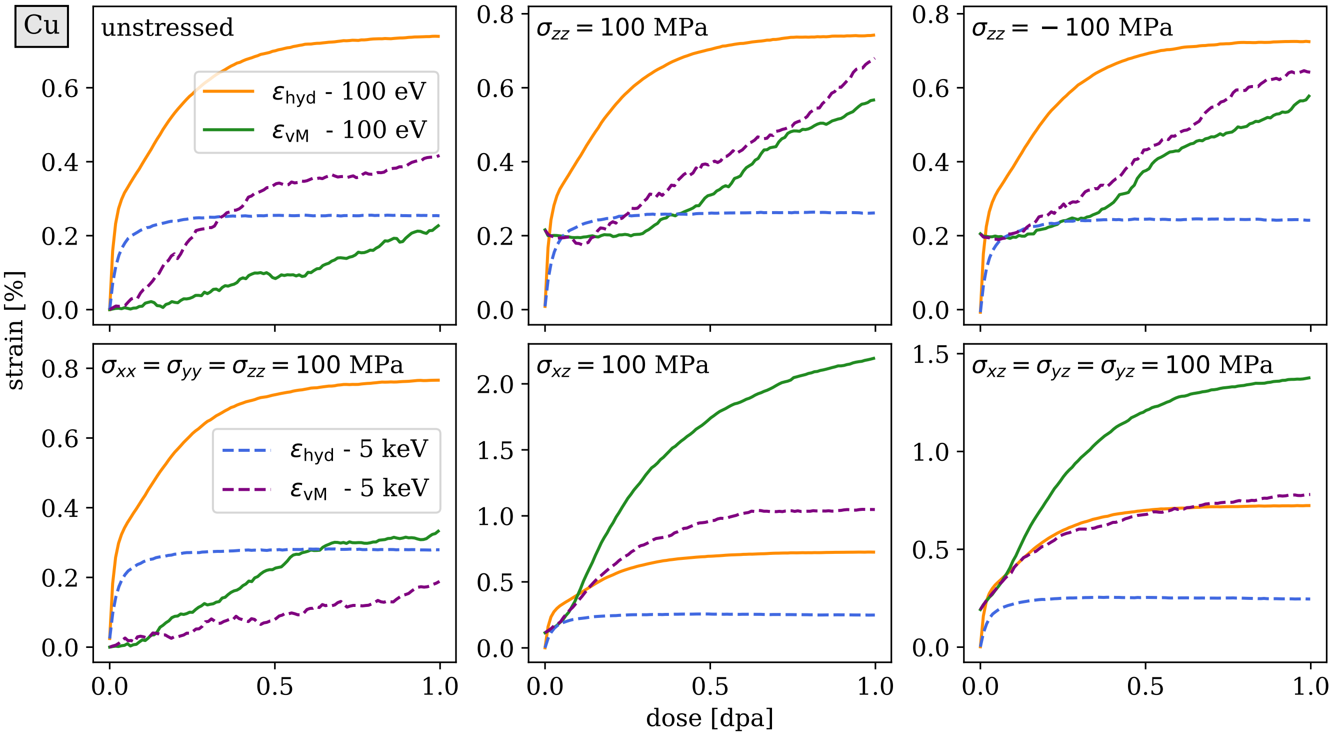


(b)

FIG. S5. Hydrostatic and von Mises strains in W (a) and in Cu (b) for low- (solid) and high-energy (dashed lines) equivalent molten spheres. Each panel has a different applied stress. Low-energy irradiation produces more defects overall and hence more radiation creep upon their re-organisation. At the zero-dose limit the elastic strains are visible and much smaller than the subsequent evolution. Note that the $y$-axes have different maximum values; the hydrostatic stresses are not very affected by the external stress.

where $\boldsymbol{\varepsilon}^{\rm el}$, $\boldsymbol{\varepsilon}^{\omega}$ and $\mathbf{R}$ are elastic strain, irreversible strain given by swelling and rotation.

In Tab. S2 we summarise the supercell strain at 1 dpa simulating 90 eV equivalent recoil energy in W and 100 eV equivalent recoil energy in Cu. Strains are divided into elastic and irreversible contributions. In all cases we find that the plastic part dominates over the elastic part. We also note that the initial elastic strain components applied through imposing the external elastic stress, namely $C^{-1}_{ijkl}\sigma_{kl}$, were of the order of 0.1 %. This is approximately the same magnitude as the values that we find at 1 dpa. In the next section we detail how the lattice strain is calculated.

### A. Strain from diffraction pattern of completing atomic planes

Consider a box of atoms, with length $A$ in the z-direction made up of $N \gg 1$ planes of atoms. The reference lattice parameter is $a_0 = A/N$. Now introduce a prismatic interstitial dislocation loop into the box, oriented with the z-direction, occupying a fraction of the plane $\rho$. When $\rho = 0$, this is the perfect crystal case with no interstitials, and $\rho = 1$ indicates perfect crystal with $N+1$ planes of atoms.

Ignoring local strains and core effects, the eigenstrain due to the dislocation loop is $\varepsilon = \rho/N$, so the box dimension with the interstitial is $A' = A(1+\varepsilon)$ The z-position of plane $j$ can be approximated as $z_j = A'j/N$, with $j \in \{0, 1, \ldots, N-1\}$ in a position outside the boundary of the dislocation loop and as $z_j = A'j/(N+1)$, with $j \in \{0, 1, \ldots, N\}$ inside the boundary. We can write down the structure factor as

$$\begin{aligned} S(k;\rho) &= \frac{(1-\rho)}{N+\rho} \sum_{j=0}^{N-1} \exp\left[-i\frac{kA'j}{N}\right] \\ &+ \frac{\rho}{N+\rho} \sum_{j=0}^{N} \exp\left[-i\frac{kA'j}{N+1}\right]. \end{aligned} \tag{13}$$

Note the denominator term $N+\rho$ is a normalising factor. Summing the geometric series, this can be reexpressed as

$$\begin{aligned} S(k;\rho) &= \frac{(1-\rho)}{N+\rho} \exp\left[-i\frac{(N-1)kA'}{2N}\right] \\ &\times \csc\left[\frac{kA'}{2N}\right] \sin\left[\frac{kA'}{2}\right] \\ &+ \frac{\rho}{N+\rho} \exp\left[-i\frac{NkA'}{2(N+1)}\right] \\ &\csc\left[\frac{kA'}{2(N+1)}\right] \sin\left[\frac{kA'}{2}\right], \end{aligned} \tag{14}$$

and so the diffraction intensity is

$$\begin{aligned} I(k;\rho) = |S(k;\rho)|^2 = \frac{\sin^2\left[\frac{kA'}{2}\right]}{(N+\rho)^2} \{ (1-\rho)^2 \csc^2\left[\frac{kA'}{2N}\right] \\ +2\rho(1-\rho)\cos\left[\frac{kA'}{2N(1+N)}\right] \csc\left[\frac{kA'}{2N}\right] \csc\left[\frac{kA'}{2+2N}\right] \\ +\rho^2 \csc^2\left[\frac{kA'}{2+2N}\right] \}. \end{aligned} \tag{15}$$

At the expected diffraction peak positions $k_1 = 2\pi N/A'$ and $k_2 = 2\pi(N+1)/A'$, the intensity has a particularly simple form:

$$I(k;\rho) = \begin{cases} \dfrac{N^2}{(N+\rho)^2}(1-\rho)^2 & k = \frac{2\pi N}{A'} \\ \dfrac{(1+N)^2}{(N+\rho)^2}\rho^2 & k = \frac{2\pi(N+1)}{A'} \end{cases} \tag{16}$$

We can therefore find an approximate peak location, $\langle k \rangle$, from the first moment of these two diffraction peaks,

$$\begin{aligned} \langle k \rangle &= \frac{k_1 I(k_1;\rho) + k_2 I(k_2;\rho)}{I(k_1;\rho) + I(k_2;\rho)} \\ &= \frac{2\pi}{A'}\left(N + \frac{\rho^2}{1-2\rho+2\rho^2} + \mathcal{O}(1/N)\right). \end{aligned} \tag{17}$$

The second term here is the critical part of this analysis. The function $f(\rho) = \rho^2/(1-2\rho+2\rho^2)$ is a sigmoid curve, smoothly transitioning from $f(0) = 0$ through $f(1/2) = 1/2$ to $f(1) = 1$. If we constrain our interpretation of the cell to be a single crystal, with an integer number of planes, then when $\rho < 1/2$ we read the number of planes as $N$. The lattice parameter is $a = A'/N$, and so we find the strain, $\varepsilon = a/a_0 - 1$ is positive:

$$\varepsilon(\rho < 1/2) = \frac{\rho}{N}. \tag{18}$$

But when $\rho > 1/2$, we read the number of planes as $N+1$, and so $a = A'/(N+1)$, and the strain is negative:

$$\varepsilon(\rho > 1/2) = -\frac{1-\rho}{N+1}. \tag{19}$$

Near the critical point $\rho = 1/2$, small fluctuations in $\rho$ could lead us to select one case or the other.

If we remove the criterion that the cell is a single crystal, we could instead say some part has $N$ planes and some part has $N+1$. The fraction with $N$ planes can be weighted by the relative intensity $I(k_1)/(I(k_1)+I(k_2))$. Then the strain is weighted accordingly, to read

$$\begin{aligned} \varepsilon &= \frac{I(k_1)\varepsilon(\rho < 1/2) + I(k_2)\varepsilon(\rho > 1/2)}{I(k_1) + I(k_2)} \\ &= \frac{\rho(2\rho-1)(\rho-1)}{N(1-2\rho+2\rho^2)} + \mathcal{O}(1/N^2). \end{aligned} \tag{20}$$

This analysis shows that it is not half-completed planes of atoms that give abrupt changes in strain, but rather the overly strict interpretation that a single crystal must prevail, when it might be better to accept from the diffraction pattern that multiple interpretations are possible.

TABLE S2. The total strain given by the deformation of the supercell, $\boldsymbol{\varepsilon}^{\mathbf{scll}}$, was calculated using Eqs. (5)-(10). It was also decomposed into elastic $\boldsymbol{\varepsilon}^{\mathbf{el}}$, irradiation-induced irreversible strain $\boldsymbol{\varepsilon}^{\boldsymbol{\omega}}$ and rotation according to the total transformation $(\mathbf{1}+\boldsymbol{\varepsilon}^{\mathrm{el}})\mathbf{R}(\mathbf{1}+\boldsymbol{\varepsilon}^{\boldsymbol{\omega}})$. The six components of strain at 1 dpa are tabulated for the three strain tensors. The plastic strain is usually much greater that the atomic strain, especially in the case of copper, and in tungsten the atomic strain is usually compressive. The hydrostatic strain invariant is also included, allowing one to note that, given the fairly small magnitudes involved, to within 1 % we have that $\varepsilon^{\mathrm{scll}}_{\mathrm{hyd}} = \varepsilon^{\mathrm{el}}_{\mathrm{hyd}} + \varepsilon^{\omega}_{\mathrm{hyd}}$. The results refer to the low equivalent recoil energy simulations.

| | Tungsten | | | | | | | | Copper | | | | | | | |
|---|---|---|---|---|---|---|---|---|---|---|---|---|---|---|---|---|
| | $\varepsilon_{xx}$ | $\varepsilon_{yy}$ | $\varepsilon_{zz}$ | $\varepsilon_{xy}$ | $\varepsilon_{yz}$ | $\varepsilon_{xz}$ | $\varepsilon_{\mathrm{hyd}}$ | | $\varepsilon_{xx}$ | $\varepsilon_{yy}$ | $\varepsilon_{zz}$ | $\varepsilon_{xy}$ | $\varepsilon_{yz}$ | $\varepsilon_{xz}$ | $\varepsilon_{\mathrm{hyd}}$ | |
| | unstressed | | | | | | | | unstressed | | | | | | | |
| $\varepsilon^{\mathrm{el}}$ | -0.18 | -0.12 | -0.31 | 0.07 | -0.07 | -0.15 | -0.20 | 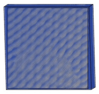 | 0.19 | 0.14 | -0.05 | 0.01 | -0.01 | -0.03 | 0.09 | 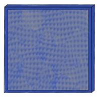 |
| $\varepsilon^{\omega}$ | 0.51 | 0.49 | 0.50 | -0.23 | -0.02 | 0.23 | 0.50 | | 0.65 | 0.63 | 0.64 | 0.00 | 0.00 | 0.01 | 0.64 | |
| $\varepsilon^{\mathrm{el}}+\varepsilon^{\omega}$ | 0.33 | 0.37 | 0.19 | -0.15 | -0.09 | 0.08 | 0.30 | | 0.84 | 0.77 | 0.59 | 0.01 | -0.01 | -0.02 | 0.74 | |
| $\varepsilon^{\mathrm{scll}}$ | 0.33 | 0.37 | 0.19 | -0.16 | -0.09 | 0.07 | 0.30 | | 0.84 | 0.78 | 0.59 | 0.01 | -0.01 | -0.02 | 0.74 | |
| | $\sigma_{zz} = 500$ MPa | | | | | | | | $\sigma_{zz} = 100$ MPa | | | | | | | |
| $\varepsilon^{\mathrm{el}}$ | -0.18 | -0.31 | -0.06 | -0.03 | -0.06 | 0.01 | -0.19 | 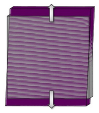 | -0.08 | -0.06 | 0.14 | 0.06 | 0.13 | 0.04 | 0.00 | 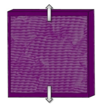 |
| $\varepsilon^{\omega}$ | 0.00 | 0.24 | 1.25 | 0.12 | 0.24 | -0.12 | 0.50 | | 0.62 | 0.64 | 0.96 | 0.00 | -0.14 | 0.00 | 0.74 | |
| $\varepsilon^{\mathrm{el}}+\varepsilon^{\omega}$ | -0.19 | -0.07 | 1.19 | 0.10 | 0.18 | -0.11 | 0.31 | | 0.54 | 0.58 | 1.10 | 0.07 | -0.01 | 0.04 | 0.74 | |
| $\varepsilon^{\mathrm{scll}}$ | -0.18 | -0.07 | 1.19 | 0.09 | 0.18 | -0.11 | 0.31 | | 0.54 | 0.58 | 1.11 | 0.07 | -0.01 | 0.04 | 0.74 | |
| | $\sigma_{zz} = -500$ MPa | | | | | | | | $\sigma_{zz} = -100$ MPa | | | | | | | |
| $\varepsilon^{\mathrm{el}}$ | -0.10 | -0.18 | -0.37 | 0.18 | -0.08 | -0.17 | -0.22 | 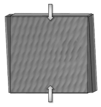 | -0.07 | 0.20 | -0.16 | 0.12 | 0.02 | -0.02 | -0.01 | 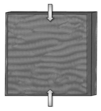 |
| $\varepsilon^{\omega}$ | 0.52 | 0.74 | 0.25 | -0.34 | 0.24 | 0.09 | 0.50 | | 0.94 | 0.63 | 0.62 | -0.31 | -0.16 | -0.01 | 0.73 | |
| $\varepsilon^{\mathrm{el}}+\varepsilon^{\omega}$ | 0.41 | 0.56 | -0.12 | -0.16 | 0.16 | -0.08 | 0.29 | | 0.87 | 0.83 | 0.46 | -0.19 | -0.14 | -0.03 | 0.72 | |
| $\varepsilon^{\mathrm{scll}}$ | 0.41 | 0.56 | -0.12 | -0.16 | 0.16 | -0.08 | 0.28 | | 0.88 | 0.84 | 0.46 | -0.19 | -0.14 | -0.03 | 0.72 | |
| | $\sigma_{xx}+\sigma_{yy}+\sigma_{zz} = 500$ MPa | | | | | | | | $\sigma_{xx}+\sigma_{yy}+\sigma_{zz} = 100$ MPa | | | | | | | |
| $\varepsilon^{\mathrm{el}}$ | -0.25 | -0.23 | -0.17 | 0.12 | -0.11 | 0.06 | -0.22 | 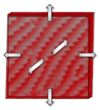 | 0.02 | -0.08 | 0.13 | -0.01 | -0.10 | 0.12 | 0.02 | 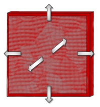 |
| $\varepsilon^{\omega}$ | 0.48 | 0.73 | 0.50 | -0.11 | 0.36 | 0.01 | 0.57 | | 0.65 | 0.92 | 0.64 | -0.15 | 0.15 | -0.14 | 0.74 | |
| $\varepsilon^{\mathrm{el}}+\varepsilon^{\omega}$ | 0.23 | 0.51 | 0.33 | 0.01 | 0.26 | 0.07 | 0.36 | | 0.67 | 0.84 | 0.78 | -0.16 | 0.05 | -0.02 | 0.76 | |
| $\varepsilon^{\mathrm{scll}}$ | 0.23 | 0.50 | 0.33 | 0.01 | 0.26 | 0.07 | 0.36 | | 0.67 | 0.85 | 0.78 | -0.16 | 0.05 | -0.02 | 0.77 | |
| | $\sigma_{xz} = 500$ MPa | | | | | | | | $\sigma_{xz} = 100$ MPa | | | | | | | |
| $\varepsilon^{\mathrm{el}}$ | -0.16 | -0.11 | -0.14 | 0.10 | -0.08 | -0.18 | -0.14 | 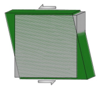 | -0.07 | -0.09 | 0.10 | -0.09 | 0.07 | -0.07 | -0.02 | 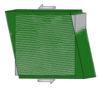 |
| $\varepsilon^{\omega}$ | 0.75 | 0.00 | 0.50 | -0.12 | 0.00 | -0.62 | 0.42 | | 0.95 | 0.29 | 0.97 | 0.15 | -0.16 | -1.09 | 0.74 | |
| $\varepsilon^{\mathrm{el}}+\varepsilon^{\omega}$ | 0.58 | -0.11 | 0.36 | -0.02 | -0.08 | -0.80 | 0.28 | | 0.88 | 0.21 | 1.07 | 0.06 | -0.09 | -1.16 | 0.72 | |
| $\varepsilon^{\mathrm{scll}}$ | 0.59 | -0.11 | 0.37 | -0.02 | -0.08 | -0.80 | 0.28 | | 0.89 | 0.21 | 1.08 | 0.06 | -0.09 | -1.17 | 0.73 | |
| | $\sigma_{xy}+\sigma_{yz}+\sigma_{xz} = 500$ MPa | | | | | | | | $\sigma_{xy}+\sigma_{yz}+\sigma_{xz} = 100$ MPa | | | | | | | |
| $\varepsilon^{\mathrm{el}}$ | -0.06 | 0.00 | -0.13 | -0.19 | -0.13 | -0.22 | -0.06 | 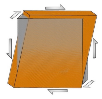 | 0.10 | 0.01 | 0.10 | 0.01 | -0.10 | -0.06 | 0.07 | 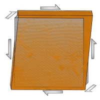 |
| $\varepsilon^{\omega}$ | 0.26 | 0.04 | 0.78 | -0.39 | -0.62 | -0.52 | 0.36 | | 0.67 | 0.64 | 0.64 | -0.44 | -0.32 | -0.45 | 0.65 | |
| $\varepsilon^{\mathrm{el}}+\varepsilon^{\omega}$ | 0.20 | 0.04 | 0.65 | -0.58 | -0.75 | -0.74 | 0.30 | | 0.77 | 0.65 | 0.74 | -0.43 | -0.42 | -0.51 | 0.72 | |
| $\varepsilon^{\mathrm{scll}}$ | 0.20 | 0.05 | 0.67 | -0.58 | -0.75 | -0.75 | 0.31 | | 0.77 | 0.65 | 0.75 | -0.43 | -0.42 | -0.51 | 0.72 | |

## V. MICROSTRUCTURAL ANALYSIS

In Fig. S6 we show the evolution of vacancy content (a) and total dislocation density (c) as a function of dose. The figure highlights that the effect of stress is limited on these two quantities, with only some effect of shear states visible. W irradiated under simple shear with an equivalent energy of 90 eV contained about 10 % fewer vacancies than the other stress states, but this was the only simulation where such a deviation was observed. The visual representation of the 1 dpa vacancy concentration is given also as a histogram in Fig. S6b. Shear states also had some effect on the dislocation density. The simplification of the network at high dose is somewhat easier under shear, this means that the decrease in dislocation density was found to be more pronounced in this case. The trend in the dislocation density follows that of irradiated materials in the athermal limit where stress-driven defect dynamics dominates [2]. In the initially dislocation-free material small dislocation loops form already at a dose $\lesssim 0.001$ dpa. This causes a sudden increase in dislocation content. The coalescence of the small loops into larger ones and then a large network is reflected in a decrease in dislocation density. Although not shown in the fig-

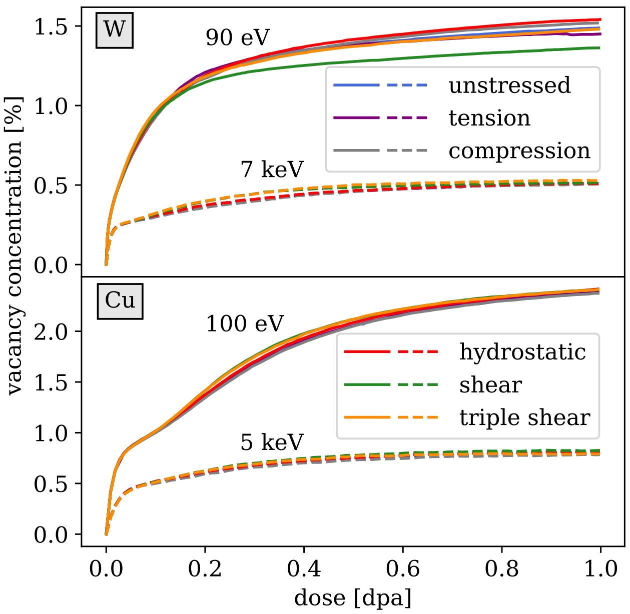


(a)

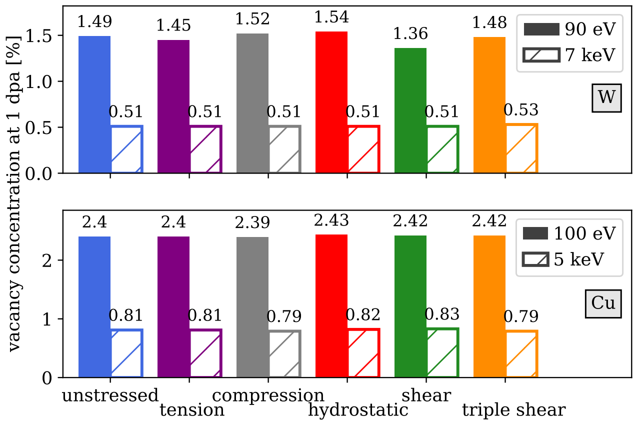


(b)

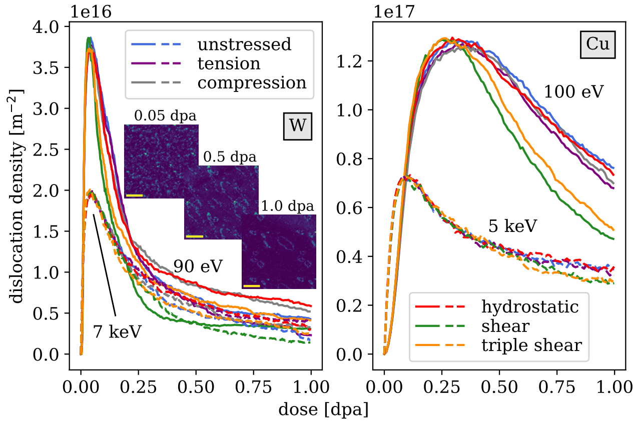


(c)

FIG. S6. (a) The vacancy concentration increases with dose towards saturation in W and Cu, upper and lower panel respectively. Equivalent cascades of higher energy produce much fewer vacancies in both metals. Interestingly, the applied stress does not strongly influence the vacancy concentration, whose value at 1 dpa is also summarised in the histograms in (b). (c) Similarly, the total dislocation density as a function of dose is highly sensitive to the PKA energy but not much affected by the stress state. Insets in (d) show dark field simulated TEM of sheared box (7 keV); scale bar is 20 nm and $\mathbf{g} = [002]$ is horizontal.

ure, also the relative predominance of different Burgers vectors in the dislocations changes with dose. In W, the high-dose limit is dominated by $1/2\langle 111\rangle$ dislocations. In Cu, the same happens for $1/6\langle 112\rangle$ Burgers vector, with the difference that there remains a dispersion of stacking fault tetrahedra (SFT) associated with $1/6\langle 110\rangle$ dislocations. The simulated TEM images of bcc-W in Fig. S6c show qualitative similarities with the dislocation evolution of ion-irradiated bcc-Fe [8].

As it was mentioned here and in the main text, irradiation of Cu produced a dispersion of SFT. An image of these tetrahedra as they appear in the simulation under shear stress is given in Fig. S7. The SFTs have a size of a few nanometres, and contain typically $\lesssim 20$ vacancies. Together with the dislocations calculated by the Ovito package, we also represent self-interstitial atoms and vacancies calculated by Wigner-Seitz analysis. A good correlation between tetrahedral-shaped dislocations having $1/6\langle 110\rangle$ Burgers vector and vacancy clusters could be found.

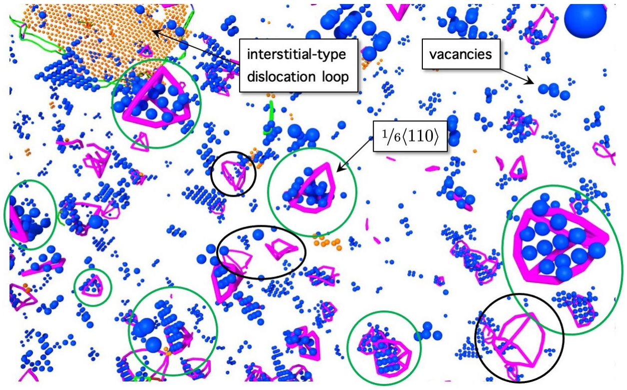


FIG. S7. 1 dpa Cu simulation under shear where dislocations, self-interstitials and vacancies (calculated by Wigner-Seitz analysis) are visualised. There is a clear correlation between stacking-fault tetrahedra and vacancy clusters (green circles) although this was not always the case (black circles). Isolated vacancies were filtered out to allow one to see through the fine dispersion of isolated vacancies.

## A. Copper irradiated to 2 dpa without applied stress

Observing the simulations of copper with respect to tungsten it is clear that the evolution of the dislocation network of copper is slower. Moreover, in Cu it seemed that the numerical values of vacancy concentration and volume swelling were very close in all 12 simulations. However, by comparing the plot of these two quantities as a function of dose one can see that the gradient is different, with volume swelling almost flat but with vacancy concentration still increasing. The simulation of unstressed copper and 100 eV equivalent recoil energy was therefore extended until 2 dpa. We can see in Fig. S8 that indeed vacancy content kept increasing, volume swelling remained broadly constant and dislocation content kept falling until 2 dpa. The fact that vacancy concentration and swelling were very close in their values at 1 dpa was coincidental. Although swelling had reached saturation by that point, vacancy concentration still had a noticeable gradient and increased by about 10 % from 1 to 2 dpa.


[1] M. Boleininger, D. R. Mason, A. E. Sand, and S. L. Dudarev, Microstructure of a heavily irradiated metal exposed to a spectrum of atomic recoils, Scientific Reports **13**, 1684 (2023).

[2] P. M. Derlet and S. L. Dudarev, Microscopic structure of a heavily irradiated material, Physical Review Materials **4**, 023605 (2020).

[3] A. Chartier and M.-C. Marinica, Rearrangement of interstitial defects in alpha-Fe under extreme condition, Acta Materialia **180**, 141 (2019).

[4] M. Boleininger, S. L. Dudarev, D. R. Mason, and E. Martínez, Volume of a dislocation network, Physical Review Materials **6**, 063601 (2022).

[5] D. R. Mason, F. Granberg, M. Boleininger, T. Schwarz-Selinger, K. Nordlund, and S. L. Dudarev, Parameter-free quantitative simulation of high-dose microstructure and hydrogen retention in ion-irradiated tungsten, Physical Review Materials **5**, 095403 (2021).

[6] D. R. Mason, S. Das, P. M. Derlet, S. L. Dudarev, A. J. London, H. Yu, N. W. Phillips, D. Yang, K. Mizohata, R. Xu, and F. Hofmann, Observation of transient and asymptotic driven structural states of tungsten exposed to radiation, Physical Review Letters **125**, 225503 (2020).

[7] M. J. Banisalman, S. Park, and T. Oda, Evaluation of the threshold displacement energy in tungsten by molecular dynamics calculations, Journal of Nuclear Materials **495**, 277 (2017).

[8] M. Hernández-Mayoral, Z. Yao, M. Jenkins, and M. Kirk, Heavy-ion irradiations of Fe and Fe–Cr model alloys part 2: Damage evolution in thin-foils at higher doses, Philosophical Magazine **88**, 2881 (2008).

[9] A. Stukowski, Visualization and analysis of atomistic simulation data with OVITO–the Open Visualization Tool, Modelling and Simulation in Materials Science and Engineering **18**, 015012 (2009).

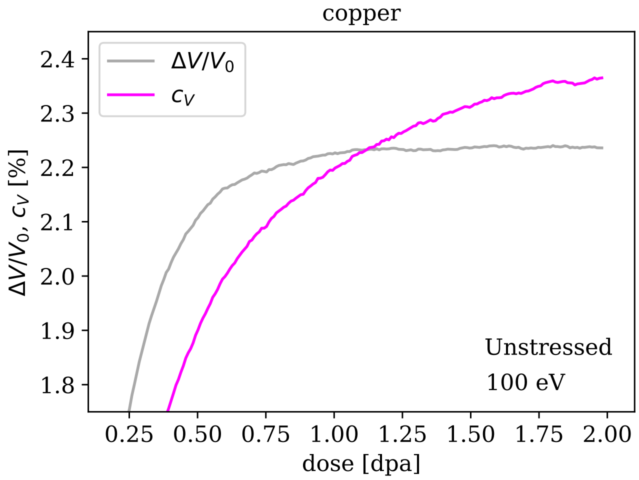


(a)

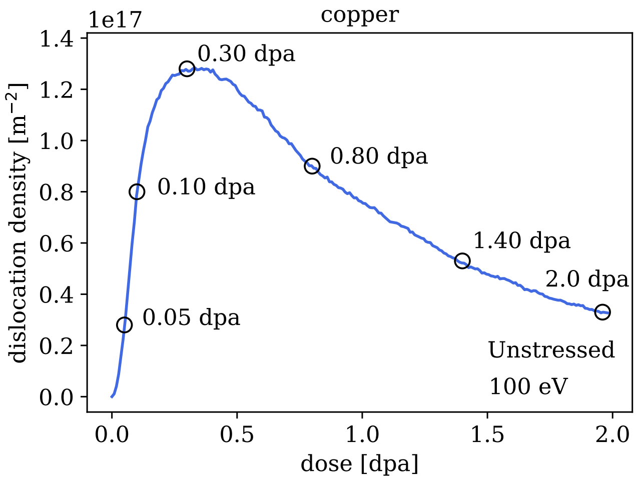


(b)

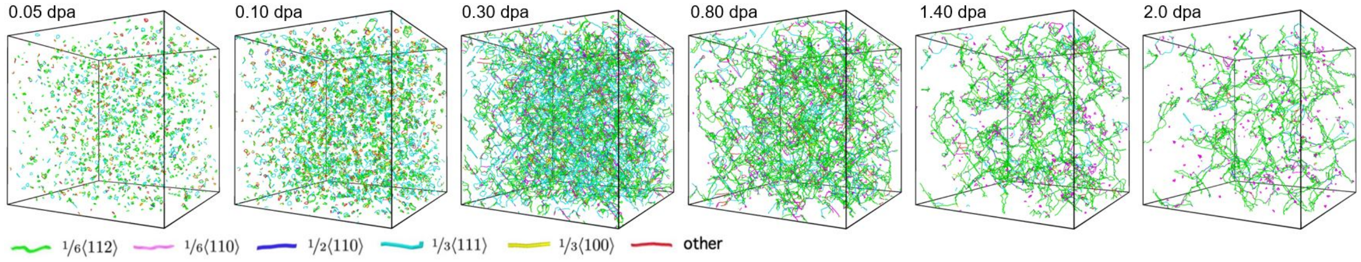


(c)

FIG. S8. The copper simulation without any external stress and using 100 eV equivalent recoil energy was extended to 2 dpa to observe the residual evolution of the microstructure in the high-dose range. (a) Vacancy concentration compared to volume swelling showing the that the latter reached saturation by 1 dpa, differently from the former. (b) Total dislocation density. Although almost at the steady state, it is apparent that vacancy concentration would still rise slightly and dislocation density would decrease slightly above 2 dpa. (c) Dislocation analysis [9] showing that after the simplification of the very complex dislocation tangle visible at 0.3 dpa the material retains an extended network of predominantly $1/6\langle 112\rangle$ Burgers vector and a dispersion of smaller dislocations of predominantly $1/6\langle 110\rangle$ Burgers vector.
